# Supplementary material for: Which Identities Are Mobilized: Towards an automated detection of social group appeals in political texts
Source: arXiv:2405.01904 source file (2024-05-03)
Supplement: Supplementary file 1 [file 9A-appendix.tex]

%----------------------------------------------------------------------------------------
% Appendix
%----------------------------------------------------------------------------------------
\newpage % Includes a new page
\section*{Appendix} % Stars disable section numbers
\addcontentsline{toc}{section}{Appendix}
